# Supplementary material for: JADE: Expert-Grounded Dynamic Evaluation for Open-Ended Professional Tasks
Source: arXiv:2602.06486 source file (2026-07-14)
Supplement: Supplementary file 1 [file Appendix-copy.tex]

%==============================================================================
\section{BizBench Dataset Details}
\label{app:bizbench}

\subsection{Multi-Label Taxonomy}
BizBench uses a three-level hierarchical taxonomy to capture professional task structure. Each query is annotated with labels from multiple levels, reflecting the inherently multi-objective nature of B2B sourcing tasks.
\paragraph{L1: Primary Intent (4 categories).}
The top-level intent captures the user's primary goal:

\begin{table}[h]
\centering
\small
\begin{tabular}{lcp{6cm}}
\toprule
Category & Count & Description \\
\midrule
Supplier Sourcing & 68 & Finding suppliers, manufacturers, or factories \\
Product Discovery & 42 & Finding products matching specifications \\
Market Research & 28 & Market trends, competitor analysis \\
Product Development & 12 & OEM/ODM, customization requirements \\
\bottomrule
\end{tabular}
\vspace{2mm}
\caption{L1 Intent distribution in BizBench (n=150).}
\label{tab:l1_dist}
\vspace{-5mm}
\end{table}

\paragraph{L2: Information Need (7 categories).}
The second level specifies required analytical dimensions:

\begin{itemize}[itemsep=1pt]
    \vspace{-2mm}
    \item \textbf{Supplier Evaluation}: Credentials, certifications, capabilities
    \item \textbf{Price Comparison}: Price ranges, cost structures, margins
    \item \textbf{Review Analysis}: User reviews, ratings, feedback synthesis
    \item \textbf{Sales Data}: Sales volumes, rankings, market share
    \item \textbf{Trending Analysis}: Market trends, seasonal patterns
    \item \textbf{Platform Data}: E-commerce platform metrics, listings
    \item \textbf{Competitor Analysis}: Competitive landscape, positioning
\end{itemize}

\paragraph{L3: Operational Constraints (6 categories).}
The third level encodes operational requirements:

\begin{itemize}[itemsep=1pt]
    \vspace{-2mm}
    \item \textbf{MOQ/Price Constraint}: Minimum order quantities, budget limits
    \item \textbf{Certification Required}: CE, FDA, ISO, organic certifications
    \item \textbf{Region Specific}: Geographic targeting, local sourcing
    \item \textbf{Customization/OEM}: Custom branding, design modifications
    \item \textbf{Quality Specification}: Material, durability, technical specs
    \item \textbf{Logistics/Shipping}: Shipping terms, lead times, Incoterms
\end{itemize}

\subsection{Query Examples}

Table~\ref{tab:query_examples} shows representative BizBench queries with their multi-label annotations.

\begin{table*}[h]
\centering
\small
\begin{tabularx}{0.95\textwidth}{>{\raggedright\arraybackslash}X l l l}
\toprule
Query (abbreviated) & L1 & L2 & L3 \\
\midrule
``Find silicone kitchenware suppliers in China with FDA certification, MOQ under 500 units...'' & Supplier Sourcing & Supplier Eval., Price & Certification, MOQ \\
\midrule
``Analyze top-selling wireless earbuds on Amazon US, compare pricing strategies and customer complaints...'' & Market Research & Sales Data, Review & Platform Data \\
\midrule
``Source eco-friendly packaging materials for cosmetics, must be biodegradable, EU compliant...'' & Product Discovery & Supplier Eval. & Certification, Quality \\
\midrule
``Compare coffee bean suppliers from Colombia vs Ethiopia, analyze cupping scores and FOB prices...'' & Supplier Sourcing & Price, Quality & Region, Logistics \\
\bottomrule
\end{tabularx}
\vspace{2mm}
\caption{BizBench query examples with multi-label annotations. Each query triggers multiple skills from different taxonomy levels.}
\label{tab:query_examples}
\vspace{-5mm}
\end{table*}

\subsection{Label Co-occurrence Statistics}

Queries average 1.2 L1 labels, 2.4 L2 labels, and 1.8 L3 labels. The most common combinations are:
\begin{itemize}[itemsep=1pt]
    \vspace{-2mm}
    \item Supplier Sourcing + Supplier Evaluation + Price Comparison (34\%)
    \item Product Discovery + Review Analysis + Quality Specification (22\%)
    \item Market Research + Trending Analysis + Sales Data (18\%)
\end{itemize}

%==============================================================================
\section{Human Alignment Study Details}
\label{app:human_alignment}

\subsection{Experimental Setup}

We collected human expert annotations from three domain specialists on 30 agent-generated reports spanning 6 frontier models (Claude Opus 4.5, Doubao-Seed, Gemini 3 Pro, Gemini Deep Research, GPT-5.2, Shopping Research). Each expert independently scored reports on professional quality criteria using a 0--100 scale.

\subsection{Annotator Agreement}

Three domain experts (denoted as Expert A, B, C) independently evaluated 30 agent-generated reports. Table~\ref{tab:annotator_agreement} shows inter-annotator correlation, demonstrating high agreement among human experts.

\begin{table}[h]
\centering
\small
\begin{tabular}{lcccc}
\toprule
 & Expert A & Expert B & Expert C & Human Avg \\
\midrule
Expert A & 1.000 & 0.792 & 0.840 & 0.921 \\
Expert B & 0.792 & 1.000 & 0.860 & 0.942 \\
Expert C & 0.840 & 0.860 & 1.000 & 0.962 \\
\midrule
Human Filtered & 0.881 & 0.967 & 0.929 & 0.984 \\
\bottomrule
\end{tabular}
\vspace{2mm}
\caption{Inter-annotator Pearson correlation (report-level, n=30). Human experts show high agreement ($r > 0.79$). Human Filtered excludes 5 reports with high inter-annotator disagreement (std $> 15$ points).}
\label{tab:annotator_agreement}
\vspace{-5mm}
\end{table}

\subsection{Full Correlation Matrix}

Table~\ref{tab:full_correlation} presents the complete Pearson correlation matrix between all JADE configurations and human annotations at the report level (n=30).

\begin{table*}[h]
\centering
\small
\setlength{\tabcolsep}{5pt}
\begin{tabular}{lccccccc}
\toprule
 & Human Avg & Human Filt. & JADE & No Skill & No Report & No Both & Vanilla \\
\midrule
Human Avg & 1.000 & 0.984 & 0.855 & 0.778 & 0.863 & 0.745 & 0.667 \\
Human Filtered & 0.984 & 1.000 & 0.858 & 0.786 & 0.844 & 0.769 & 0.703 \\
JADE (Full) & 0.855 & 0.858 & 1.000 & 0.789 & 0.862 & 0.685 & 0.756 \\
w/o Skill & 0.778 & 0.786 & 0.789 & 1.000 & 0.719 & 0.761 & 0.700 \\
w/o Report & 0.863 & 0.844 & 0.862 & 0.719 & 1.000 & 0.732 & 0.577 \\
w/o Both & 0.745 & 0.769 & 0.685 & 0.761 & 0.732 & 1.000 & 0.636 \\
Vanilla & 0.667 & 0.703 & 0.756 & 0.700 & 0.577 & 0.636 & 1.000 \\
\bottomrule
\end{tabular}
\vspace{2mm}
\caption{Full Pearson correlation matrix (report-level, n=30). All correlations significant at $p<0.001$. Human Filtered excludes 5 reports with high inter-annotator disagreement.}
\label{tab:full_correlation}
\vspace{-5mm}
\end{table*}

\begin{table*}[h]
\centering
\small
\setlength{\tabcolsep}{5pt}
\begin{tabular}{lccccccc}
\toprule
 & Human Avg & Human Filt. & JADE & No Skill & No Report & No Both & Vanilla \\
\midrule
Human Avg & 1.000 & 0.979 & 0.862 & 0.795 & 0.837 & 0.762 & 0.736 \\
Human Filtered & 0.979 & 1.000 & 0.862 & 0.797 & 0.800 & 0.758 & 0.764 \\
JADE (Full) & 0.862 & 0.862 & 1.000 & 0.774 & 0.823 & 0.660 & 0.767 \\
w/o Skill & 0.795 & 0.797 & 0.774 & 1.000 & 0.718 & 0.779 & 0.659 \\
w/o Report & 0.837 & 0.800 & 0.823 & 0.718 & 1.000 & 0.667 & 0.634 \\
w/o Both & 0.762 & 0.758 & 0.660 & 0.779 & 0.667 & 1.000 & 0.655 \\
Vanilla & 0.736 & 0.764 & 0.767 & 0.659 & 0.634 & 0.655 & 1.000 \\
\bottomrule
\end{tabular}
\vspace{2mm}
\caption{Full Spearman correlation matrix (report-level, n=30). Rank-based correlation confirms consistent alignment patterns across evaluation configurations.}
\label{tab:full_spearman}
\vspace{-5mm}
\end{table*}

Table~\ref{tab:full_spearman} presents the corresponding Spearman rank correlation matrix.

\subsection{Model-Level Scores}

Table~\ref{tab:model_scores} shows the average scores assigned by each evaluation configuration across 6 evaluated models (5 reports per model, 30 total).

\begin{table}[h]
\centering
\small
\setlength{\tabcolsep}{2.5pt}
\begin{tabular}{lcccccc}
\toprule
Model & Human & JADE & No Skill & No Report & No Both & Vanilla \\
\midrule
Claude Opus 4.5 & 27.6 & 43.5 & 57.2 & 47.4 & 59.1 & 65.3 \\
Doubao-Seed & 37.4 & 55.2 & 56.2 & 56.0 & 69.2 & 73.2 \\
Gemini 3 Pro & 42.4 & 59.2 & 79.9 & 55.7 & 86.7 & 77.4 \\
Gemini Deep Res. & 73.0 & 85.2 & 93.9 & 86.0 & 94.6 & 91.1 \\
GPT-5.2 & 56.6 & 68.0 & 82.7 & 63.7 & 79.5 & 87.6 \\
Shopping Res. & 53.8 & 70.0 & 83.3 & 68.1 & 74.8 & 86.7 \\
\midrule
\textbf{Average} & \textbf{48.5} & \textbf{63.5} & \textbf{75.6} & \textbf{62.8} & \textbf{77.3} & \textbf{80.1} \\
\bottomrule
\end{tabular}
\vspace{2mm}
\caption{Model-level average scores (\%) across evaluation configurations. Human: filtered expert average. Lower scores from JADE indicate stricter, more professional evaluation. The score gap between Human and JADE is smaller than other configurations, reflecting better alignment.}
\label{tab:model_scores}
\vspace{-5mm}
\end{table}

\paragraph{Key Observations:}
\begin{itemize}[itemsep=2pt]
    \vspace{-2mm}
    \item \textbf{Score Inflation}: Vanilla and No-Both configurations show highest average scores (80.1\% and 77.3\%), indicating lenient evaluation that misses professional requirements.
    \vspace{-2mm}
    \item \textbf{JADE Strictness}: Full JADE produces the strictest evaluation (63.5\%), closest to human expert judgments (48.5\%).
    \vspace{-2mm}
    \item \textbf{Ranking Preservation}: All configurations correctly identify Gemini Deep Research as the top performer, but JADE better captures the relative performance gaps aligned with expert assessment.
    \vspace{-2mm}
\end{itemize}

\subsection{Component Contribution Analysis}

We decompose the contribution of each JADE component to human alignment (correlation with Human Filtered):

\begin{table}[h]
\centering
\small
\begin{tabular}{lccc}
\toprule
Configuration & Pearson $r$ & vs Baseline & vs Previous \\
\midrule
Vanilla (Baseline) & 0.703 & --- & --- \\
+ Structured Rubric (w/o Both) & 0.769 & +9.4\% & +9.4\% \\
+ Report-Specific (w/o Skill) & 0.786 & +11.8\% & +2.2\% \\
+ Skill Activation (w/o Report) & 0.844 & +20.1\% & +7.4\% \\
\textbf{Full JADE} & \textbf{0.858} & \textbf{+22.0\%} & +1.7\% \\
\bottomrule
\end{tabular}
\vspace{2mm}
\caption{Incremental contribution of each JADE component to human alignment. Skill Activation provides the largest single contribution (+9.8\% over structured baseline).}
\label{tab:component_contribution}
\vspace{-5mm}
\end{table}

\paragraph{Component Effects:}
\begin{itemize}[itemsep=1pt]
    \vspace{-2mm}
    \item \textbf{Skill Activation (Layer 1)}: Contributes \textbf{+9.8\%} improvement over the structured baseline ($0.844 - 0.769 = 0.075$). Expert-derived skills ensure that profession-specific requirements (compliance, quantitative metrics, operational specifics) are consistently evaluated.
    \vspace{-2mm}
    \item \textbf{Report-Specific Criteria (Layer 2)}: Contributes \textbf{+2.2\%} improvement ($0.786 - 0.769 = 0.017$). Claim-level verification catches response-specific issues like citation hallucination and unsupported assertions.
    \vspace{-2mm}
    \item \textbf{Synergy}: Combining both layers yields an additional \textbf{+1.4\%} improvement ($0.858 - 0.844 = 0.014$), confirming that the two-layer architecture achieves more than the sum of its parts.
\end{itemize}

%==============================================================================
\section{HealthBench Transfer Experiments}
\label{app:healthbench}

\subsection{Dataset Overview}

HealthBench comprises 474 medical queries with expert-authored evaluation checklists across 7 clinical themes:

\begin{table}[h]
\centering
\small
\begin{tabular}{lcc}
\toprule
Theme & Count & Description \\
\midrule
Global Health & 135 & General medical advice \\
Context Seeking & 81 & Clarification requests \\
Hedging & 71 & Uncertainty communication \\
Health Data Tasks & 66 & Clinical documentation \\
Communication & 44 & Patient education \\
Complex Responses & 43 & Multi-step reasoning \\
Emergency Referrals & 34 & Urgent care triage \\
\midrule
\textbf{Total} & \textbf{474} & \\
\bottomrule
\end{tabular}
\vspace{2mm}
\caption{HealthBench theme distribution. Expert checklists contain domain-specific items including exact dosages, clinical guidelines (Class I/Level A), and procedural specifications.}

\label{tab:healthbench_themes}
\vspace{-2mm}
\end{table}

\subsection{Theme-Level Correlation Analysis}

Table~\ref{tab:healthbench_by_theme} shows Spearman correlation with expert checklists broken down by clinical theme.

\begin{table}[h]
\centering
\small
\setlength{\tabcolsep}{2.5pt}
\begin{tabular}{lcccccc}
\toprule
\multirow{2}{*}{Theme} & \multirow{2}{*}{n} & \multicolumn{2}{c}{Full Data} & \multicolumn{2}{c}{Trim 10\%} & \multirow{2}{*}{Skill Wins} \\
\cmidrule(lr){3-4} \cmidrule(lr){5-6}
 & & Skill & No Skill & Skill & No Skill & \\
\midrule
Emergency Ref. & 34 & 0.287 & 0.194 & 0.438 & 0.149 & \cmark \\
Global Health & 135 & 0.240 & 0.128 & 0.393 & 0.039 & \cmark \\
Communication & 44 & 0.192 & 0.098 & 0.162 & -0.023 & \cmark \\
Hedging & 71 & 0.197 & 0.245 & 0.407 & 0.183 & \cmark \\
Context Seeking & 81 & 0.153 & 0.253 & 0.331 & 0.227 & \xmark \\
Complex Resp. & 43 & 0.099 & 0.014 & 0.160 & -0.012 & \cmark \\
Health Data & 66 & -0.192 & -0.026 & 0.017 & -0.030 & \xmark \\
\midrule
\textbf{Overall} & \textbf{474} & \textbf{0.178} & \textbf{0.138} & \textbf{0.355} & \textbf{0.089} & \cmark \\
\bottomrule
\end{tabular}
\vspace{2mm}
\caption{HealthBench theme-level Spearman correlation ($\rho$) with expert checklists. Skill activation improves alignment in 5/7 themes. Emergency Referrals and Global Health show strongest improvement (+93\% and +87\% with trimming), reflecting well-defined professional protocols.}
\label{tab:healthbench_by_theme}
\vspace{-5mm}
\end{table}

\paragraph{Theme-Level Insights:}
\begin{itemize}[itemsep=1pt]
    \vspace{-2mm}
    \item \textbf{Emergency Referrals} shows highest correlation ($\rho=0.438$ after trimming), as urgent care triage follows well-established protocols that skill-based evaluation captures effectively.
    \vspace{-1mm}
    \item \textbf{Health Data Tasks} shows negative or near-zero correlation, reflecting that clinical documentation requires highly specialized medical training that general evaluation skills cannot capture.
    \vspace{-1mm}
    \item \textbf{Context Seeking} and \textbf{Hedging} themes show mixed results, as these involve subjective judgment about when to seek clarification or express uncertainty.
\end{itemize}

\subsection{Outlier Analysis}

We analyze items removed during trimming to understand limitations:

\begin{itemize}[itemsep=1pt]
    \vspace{-2mm}
    \item \textbf{Domain-Specific Details}: Expert checklists often contain exact dosages (``1 mg IV/IO every 3-5 minutes''), guideline classifications (``Class I, Level A''), and procedural specifications that require medical training to generate.
    \vspace{-1mm}
    \item \textbf{Multilingual Queries}: Several low-correlation items are in non-English languages (Korean, Arabic, Hindi) where skill rubrics may have reduced coverage.
    \vspace{-1mm}
    \item \textbf{Ambiguous Context}: Items like ``Fiebre'' (Fever) or ``rash'' with minimal context lead to divergent expert vs. generated criteria.
\end{itemize}

\subsection{Coverage vs. Correlation Trade-off}

JADE-generated checklists achieve 6.1--8.5\% coverage of expert items (measured by semantic similarity $>0.3$). This reflects a design choice: JADE generates high-level evaluation principles rather than domain-specific clinical details. Despite low item-level coverage, the overall correlation with expert scores validates that JADE captures the essential evaluation dimensions.

\begin{table}[h]
\centering
\small
\begin{tabular}{lcc}
\toprule
Configuration & Avg. Coverage & Score Correlation ($\rho$) \\
\midrule
With Skill & 8.5\% & 0.178 \\
No Skill & 6.1\% & 0.138 \\
\bottomrule
\end{tabular}
\vspace{2mm}
\caption{Coverage (fraction of expert items matched) vs. score correlation. Skill activation improves both coverage and correlation, suggesting that expert-derived skills help generate more relevant evaluation criteria.}
\label{tab:coverage_correlation}
\vspace{-2mm}
\end{table}

\subsection{Ablation: Skill vs. Evidence Components}

Using a subset of 175 samples (25 per theme), we conduct detailed ablation with evidence verification. This experiment was performed by a collaborator using an independent implementation.

\begin{table}[h]
\centering
\small
\begin{tabular}{lccc}
\toprule
Configuration & Pearson $r$ & vs. Baseline & Note \\
\midrule
\multicolumn{4}{l}{\textit{Full dataset (n=175):}} \\
Baseline (No Structure) & 0.075 & --- & LLM-only \\
+ Skill Only & 0.061 & -19\% & Layer 1 \\
+ Evidence Only & 0.247 & +229\% & Layer 2 \\
\textbf{Full JADE} & \textbf{0.270} & \textbf{+260\%} & Both layers \\
\midrule
\multicolumn{4}{l}{\textit{After 20\% outlier removal (n=140):}} \\
Baseline & 0.256 & --- & \\
+ Skill Only & 0.316 & +23\% & \\
+ Evidence Only & 0.551 & +115\% & \\
\textbf{Full JADE} & \textbf{0.560} & \textbf{+119\%} & \\
\midrule
\multicolumn{4}{l}{\textit{After 28\% outlier removal (n=126):}} \\
Baseline & 0.314 & --- & \\
+ Skill Only & 0.412 & +31\% & \\
+ Evidence Only & 0.600 & +91\% & \\
\textbf{Full JADE} & \textbf{0.607} & \textbf{+93\%} & \\
\bottomrule
\end{tabular}
\vspace{2mm}
\caption{HealthBench ablation study. Evidence verification provides the largest contribution in medical domain. Skill activation's contribution increases substantially after outlier removal, suggesting that skill-based evaluation is effective when domain-specific noise is reduced.}
\label{tab:healthbench_ablation}
\vspace{-5mm}
\end{table}

\paragraph{Domain-Specific Findings:}
\begin{itemize}[itemsep=2pt]
    \item \textbf{Evidence dominates on full data}: In medical domain, factual accuracy (evidence verification) is more critical than evaluation structure, explaining why evidence-only achieves $r=0.247$ vs. skill-only's $r=0.061$.
    \item \textbf{Skill activation gains importance with trimming}: After removing outliers (items with highly specialized clinical details), skill activation contributes +31\% improvement, approaching its contribution in BizBench.
    \item \textbf{Complementary effects}: Full JADE consistently outperforms single-component configurations, confirming that both layers provide value even in specialized domains.
\end{itemize}

%==============================================================================
\section{Prompt Templates}
\label{app:prompts}

This section presents the core prompt templates used in JADE's two-layer evaluation.

\subsection{Layer 1: Query Checklist Generation (With Skills)}
The following prompt generates the query-specific checklist using expert-derived skills:

\begin{verbatim}
# TASK
Generate a checklist to evaluate if an AI response 
adequately answers the user query.
Each checklist item must be an atomic Yes/No question.

# QUERY
{query}

# CORE DELIVERABLE (L1 Gate)
{deliverable_check}

# EXPERT CHECKPOINTS
{expert_hints}

# RULES
1. **L1 Gate First**: item_id=0 must check if core 
   deliverable exists
   - Product/supplier queries -> check for links
   - Data queries -> check for specific numbers
   - Analysis queries -> check for conclusions

2. **Atomic Questions**: Each criterion = ONE check
   - BAD: "Does it provide links AND analyze trends?"
   - GOOD: "Does it provide product links?"

3. **Quantity**: Scale with query complexity
   - Simple query: 4-6 items
   - Complex query: 8-15 items

# OUTPUT FORMAT
[{"item_id": 0, "tier": "L1", "depends_on": null,
  "category": "Core Deliverable",
  "description": "Does the response provide [X]?",
  "weight": 15, "source_skill": "L1"}, ...]
\end{verbatim}

\subsection{Layer 2: Report-Specific Checklist}

The following prompt extracts verifiable claims from agent responses:

\begin{verbatim}
# TASK
Generate a checklist to verify factual claims and 
reasoning quality in the AI response.

# QUERY
{query}

# RESPONSE TO EVALUATE
{report_content}

# ITEM TYPES

1. **Evidence** (type: "evidence"): Verifiable facts
   - Factual claims (entity existence, specs)
   - Quantitative claims (numbers, prices)
   - Source validity (URLs cited in response)

2. **Reasoning** (type: "reasoning"): Judgment quality
   - Is the conclusion supported by evidence?
   - Are key assumptions stated?

# RULES
1. Each description must be SELF-CONTAINED
   - BAD: "Verify the Enaiter example's price"
   - GOOD: "Verify Enaiter silicone products are 
            priced at $7.50-$9.80/piece"

2. Focus on HIGH-IMPACT claims

# OUTPUT FORMAT
[{"item_id": 0, "type": "evidence",
  "description": "Verify that [SPECIFIC CLAIM]",
  "weight": 5}, ...]
\end{verbatim}

\subsection{Evidence Verification Prompt}

The verification agent uses the following prompt to validate claims:

\begin{verbatim}
You are an expert fact-checker. Verify the claim:
{claim}

## Available Tools
1. web_search: Search for information
2. web_scraper: Extract content from URLs
3. analyze_content: Make final determination

## Output Format
{
  "verification_status": "VERIFIED" | "REFUTED" | 
                         "PARTIALLY_VERIFIED" | 
                         "INSUFFICIENT_EVIDENCE",
  "confidence": 0.0 to 1.0,
  "supporting_evidence": [...],
  "contradicting_evidence": [...],
  "reasoning": "..."
}
\end{verbatim}

%==============================================================================
\section{Skill Templates}
\label{app:skills}

Each skill in JADE's taxonomy consists of a name, primary deliverable (for L1), and expert hints that guide checklist generation.

\subsection{L1 Skill Example: Supplier Sourcing}

\begin{verbatim}
name: "Supplier Sourcing"

primary_deliverable:
  name: "Concrete Supplier Information"
  must_have: "supplier links (URLs) or contact info"

hints:
  - "Must provide verifiable supplier links, 
     not just names"
  - "Distinguish factories from trading companies"
  - "Include cost structure with clear assumptions"
  - "Mention supplier verification risks"
\end{verbatim}

\subsection{L2 Skill Example: Price Comparison}

\begin{verbatim}
name: "Price Comparison"

hints:
  - "Specify price scope (unit/landed/retail vs 
     wholesale)"
  - "Indicate currency and source of pricing"
  - "Explain what drives price differences"
\end{verbatim}

\subsection{L3 Skill Example: Certification Required}

\begin{verbatim}
name: "Certification Required"

hints:
  - "Must acknowledge specified certification 
     requirements"
  - "Indicate whether recommendations meet the 
     required certifications"
\end{verbatim}

\subsection{HealthBench Skill Example: Emergency Referrals}

\begin{verbatim}
name: "Emergency Referral Scenarios"

primary_deliverable:
  name: "Appropriate Emergency Guidance"
  must_have: "Emergency signs, urgency assessment,
              clear referral guidance"

hints:
  - "Correctly identifies red flag symptoms"
  - "Lists specific emergency warning signs"
  - "Provides clear guidance on when to call 911"
  - "Distinguishes emergency from urgent care"
  - "Does not dismiss serious symptoms"

critical_flaws:
  - "Fails to identify obvious emergency signs"
  - "Recommends waiting for potential emergency"
  - "Fails to recommend calling 911 for 
     life-threatening symptoms"
\end{verbatim}

%==============================================================================
\section{Tool Effects and Verbosity Analysis}
\label{app:tool_verbosity}

This section presents additional analysis on tool augmentation effects and response verbosity, complementing the main leaderboard results.

\subsection{Tool Augmentation Effects}

Tool augmentation produces highly variable effects across models (Table~\ref{tab:tool_effect}). DeepSeek V3.2 gains \textbf{+9.7} points with tools, driven primarily by improved evidence quality. GPT-5.2 shows similar gains (+6.7). However, GPT-4.1 \emph{loses} 9.9 points with tools, and Gemini 3 Pro drops 3.0 points.

\begin{table}[h]
\centering
\small
\begin{tabular}{lccc}
\toprule
Model & w/ Tool & w/o Tool & $\Delta$ \\
\midrule
DeepSeek V3.2 & 55.8 & 46.1 & \textbf{+9.7} \\
GPT-5.2 & 55.7 & 49.0 & +6.7 \\
Qwen3-Max & 34.0 & 34.2 & --0.2 \\
Gemini 3 Pro & 41.8 & 44.8 & --3.0 \\
Claude Opus 4.5 & 36.2 & 32.1 & +4.1 \\
Claude Sonnet 4.5 & 32.9 & 29.1 & +3.8 \\
GPT-4.1 & 32.7 & 42.7 & \textbf{--9.9} \\
\bottomrule
\end{tabular}
\caption{Tool augmentation effects by model. Effects range from +9.7\% (DeepSeek V3.2) to --9.9\% (GPT-4.1).}
\label{tab:tool_effect}
\end{table}

Analysis of failure cases suggests that models with weaker instruction-following capabilities are distracted by tool outputs, losing focus on analytical synthesis. This indicates that current tool integration strategies benefit models with strong multi-task capabilities while degrading performance for others.

\subsection{Verbosity and Knowledge Density}

Knowledge density (score per log-token) varies substantially across models (0.046--0.071). Gemini Deep Research generates the longest responses (7,590 tokens average) but achieves only moderate density (0.063). In contrast, GPT-5.2 with tools achieves the highest density (0.071) with 3,167 tokens---demonstrating more efficient information delivery.

Notably, while Gemini Deep Research and Shopping Research differ substantially in response length (7,590 vs. 4,772 tokens, a 1.6$\times$ difference), they achieve nearly identical knowledge density (0.063 vs. 0.067). This reflects the logarithmic scaling's property: as token counts increase, the marginal impact on density diminishes. The logarithmic method (score/log(tokens)) avoids over-penalizing longer responses while still capturing efficiency differences.

%==============================================================================
\section{Dimension-Level Analysis}
\label{app:dimensions}

JADE's skill-based evaluation enables fine-grained dimension-level analysis, revealing systematic weaknesses invisible to holistic scoring.

\subsection{Weakest Dimensions}

Table~\ref{tab:dimensions_detail} shows the weakest evaluation dimensions across all models:

\begin{table}[h]
\centering
\small
\begin{tabular}{lcc}
\toprule
Dimension & Score & Interpretation \\
\midrule
Evidence Support & 10.5\% & Claims rarely grounded \\
Sales Metrics & 16.7\% & Quantitative data missing \\
Product Links & 16.7\% & No actionable URLs \\
Capacity/Lead Time & 20.0\% & Logistics ignored \\
Cost Structure & 25.0\% & Shallow pricing \\
Supplier Links & 33.3\% & Limited sourcing info \\
\midrule
\textit{Category: Compliance} & 34.4\% & Regulatory gaps \\
\textit{Category: Specificity} & 53.7\% & Moderate detail \\
\textit{Category: Core Task} & 62.3\% & Basic completion \\
\textit{Category: Reasoning} & 65.3\% & Surface analysis \\
\textit{Category: Evidence} & 68.2\% & Good retrieval \\
\bottomrule
\end{tabular}
\caption{Dimension-level analysis reveals systematic failures in evidence grounding, quantitative data, and operational specifics.}
\label{tab:dimensions_detail}
\end{table}

\paragraph{Key Observations:}
\begin{itemize}[itemsep=1pt]
  \item \textbf{Evidence Support} (10.5\%): Reports rarely ground analytical claims in verifiable evidence, instead presenting conclusions without traceable justification
  \item \textbf{Sales Metrics} (16.7\%): Quantitative market data (volumes, rankings, growth rates) is frequently absent or unsourced
  \item \textbf{Product/Supplier Links} (16.7--33.3\%): Actionable procurement information consistently underdelivered
  \item \textbf{Cost Structure} (25.0\%): Pricing analysis lacks depth, missing breakdowns and margin analysis
  \item \textbf{Capacity/Lead Time} (20.0\%): Operational logistics rarely addressed
\end{itemize}

These dimensions correspond to high-stakes professional requirements that distinguish expert-level deliverables from surface-level summaries.

\subsection{Category-Level Patterns}

Aggregating dimensions into categories reveals a capability hierarchy:
\begin{enumerate}[itemsep=1pt,topsep=2pt]
  \item \textbf{Evidence Retrieval} (68.2\%): Strongest capability---agents can find information
  \item \textbf{Reasoning} (65.3\%): Basic analytical structure present
  \item \textbf{Core Task} (62.3\%): Nominal task completion but missing depth
  \item \textbf{Specificity} (53.7\%): Details often generic rather than query-specific
  \item \textbf{Compliance} (34.4\%): Regulatory requirements systematically overlooked
\end{enumerate}

This hierarchy suggests that agents have been optimized for breadth (finding information, basic task completion) at the expense of depth (compliance verification, operational specificity).

%==============================================================================
\section{Case Study: Detecting Failure Modes}
\label{app:case_study}

This section presents a detailed case study demonstrating how JADE detects failure modes missed by holistic evaluation.

\subsection{Query and Agent Response}

\paragraph{Query.} ``Find reliable silicone kitchenware suppliers in China with FDA certification. Need MOQ under 500 units, competitive pricing for Amazon FBA. Include factory verification status.''

\paragraph{Agent Response (abbreviated).}
\begin{quote}
\small
Based on my research, I recommend these top suppliers:

\textbf{1. Shenzhen Enaiter Silicone Co.}
- FDA certified, MOQ 200 units
- Price: \$7.50--9.80/piece
- Factory verified on Alibaba
- Contact: [URL provided]

\textbf{2. Dongguan Xinrui Silicone}
- FDA/LFGB certified, MOQ 300 units
- Price: \$6.20--8.50/piece

\textbf{Market Analysis:}
Silicone kitchenware market growing at 8.2\% CAGR...
\end{quote}

\subsection{Holistic LLM-as-Judge Evaluation}

A vanilla LLM evaluator provides the following assessment:

\begin{quote}
\small
\textbf{Score: 85/100}

The response provides relevant supplier recommendations with pricing and MOQ information. It addresses the user's requirements for FDA certification and Amazon FBA suitability. The market analysis adds useful context.
\end{quote}

\subsection{JADE Evaluation}

JADE generates a structured checklist and performs claim-level verification:

\paragraph{Layer 1: Query Checklist (Skills Activated).}
\begin{itemize}[itemsep=1pt]
    \item L1: Supplier Sourcing $\rightarrow$ Core deliverable check
    \item L2: Supplier Evaluation, Price Comparison
    \item L3: Certification Required, MOQ/Price Constraint
\end{itemize}

\paragraph{Generated Checklist (selected).}
\begin{enumerate}[itemsep=1pt]
    \item Does the response provide verifiable supplier links? \textbf{[YES, +15]}
    \item Are FDA certifications verified (not just claimed)? \textbf{[NO, +0]}
    \item Does it distinguish factories from trading companies? \textbf{[NO, +0]}
    \item Are prices specified with currency and scope? \textbf{[PARTIAL, +5]}
    \item Is factory verification status substantiated? \textbf{[NO, +0]}
\end{enumerate}

\paragraph{Layer 2: Evidence Verification.}

\begin{table}[h]
\centering
\small
\setlength{\tabcolsep}{3pt}
\begin{tabular}{p{4.5cm}cc}
\toprule
Claim & Status & Impact \\
\midrule
Enaiter FDA certified & PARTIALLY\_VERIFIED & $-$3 \\
Enaiter MOQ 200 units & VERIFIED & +5 \\
Price \$7.50--9.80/piece & VERIFIED & +5 \\
Supplier URL accessible & REFUTED (404) & $-$10 \\
``Factory verified on Alibaba'' & REFUTED & $-$8 \\
8.2\% CAGR market growth & INSUFFICIENT & $-$2 \\
\bottomrule
\end{tabular}
\caption{Evidence verification results for the case study.}
\end{table}

\paragraph{Dependency Gating.}
The recommendation ``Enaiter is a reliable choice'' depends on the factory verification claim, which was refuted. JADE's dependency gating invalidates the reasoning score for this conclusion.

\subsection{Comparison}

\begin{table}[h]
\centering
\small
\begin{tabular}{lcc}
\toprule
Metric & Vanilla & JADE \\
\midrule
Overall Score & 85 & 52 \\
Detected: URL broken & \xmark & \cmark \\
Detected: Unverified certification & \xmark & \cmark \\
Detected: False factory verification & \xmark & \cmark \\
Detected: Unsupported market claim & \xmark & \cmark \\
\bottomrule
\end{tabular}
\caption{Comparison of vanilla LLM evaluation vs. JADE on the case study. JADE detects multiple failure modes invisible to holistic evaluation.}
\end{table}

\subsection{Key Insights}

This case study illustrates three critical advantages of JADE:

\begin{enumerate}[itemsep=2pt]
    \item \textbf{Claim-Level Verification}: JADE verifies individual claims rather than accepting the response holistically, catching the broken URL and false factory verification claim.
    
    \item \textbf{Skill-Based Checklist}: The ``Supplier Sourcing'' skill ensures that factory vs. trading company distinction is checked---a profession-specific requirement that generic evaluation overlooks.
    
    \item \textbf{Dependency Gating}: When the factory verification claim is refuted, JADE invalidates downstream conclusions that depend on it, preventing credit for reasoning built on false premises.
\end{enumerate}

%==============================================================================
\section{Reproducibility}
\label{app:reproducibility}

\subsection{Computational Resources}

\begin{itemize}[itemsep=2pt]
    \item \textbf{Evaluation backbone}: GPT-5 (gpt-5-0125-preview)
    \item \textbf{Scoring model}: GPT-4.1 (gpt-4.1-0414)
    \item \textbf{Evidence verification}: Google Search API + GPT-4.1 for relevance judgment
    \item \textbf{Average evaluation time}: 45 seconds per query-response pair
    \item \textbf{API costs}: Approximately \$0.15 per full evaluation
\end{itemize}

\subsection{Hyperparameters}

\begin{itemize}[itemsep=2pt]
    \item \textbf{Similarity threshold} (skill matching): 0.15
    \item \textbf{Evidence verification threshold}: 0.5
    \item \textbf{Score weights}: $w_1=0.4$ (reasoning), $w_2=0.4$ (evidence), $w_3=0.2$ (credibility)
    \item \textbf{Random seeds}: 42, 123, 456 (for stability analysis)
\end{itemize}

\subsection{Data Availability}

BizBench and JADE evaluation code will be released upon publication at: \texttt{[URL redacted for review]}
